# Supplementary material for: Development of an Optimized Parameter Set for Monovalent Ions in the Reference Interaction Site Model of Solvation
Source: arXiv:2509.22430 ancillary file (2026-04-07)
Supplement: Supplementary file 1 [file SupplementaryMaterial.pdf]

# Supplementary Material for: Development of an Optimized Parameter Set for Monovalent Ions in the Reference Interaction Site Model of Solvation

Felipe Silva Carvalho,<sup>1</sup> Alexander McMahon,<sup>2</sup> David A. Case,<sup>3</sup> and Tyler Luchko<sup>1</sup>

<sup>1</sup>*Department of Physics and Astronomy, California State University, Northridge, Northridge, CA 91330<sup>a</sup>*

<sup>2</sup>*Department of Mathematics, California State University, Northridge, Northridge, CA 91330*

<sup>3</sup>*Department of Chemistry and Chemical Biology, Rutgers University, Piscataway, NJ 08854*

(Dated: September 23, 2025)

## I. MEAN ACTIVITY COEFFICIENT DERIVATION

The chemical potential for a system can be calculated from the Kirkwood charging formula<sup>1</sup>

$$\mu = \mu^{\text{id}} + \mu^{\text{ex}} = \mu^{\text{id}} + \int_0^1 \left\langle \frac{\partial U(r; \lambda)}{\partial \lambda} \right\rangle d\lambda$$

in which  $\langle \dots \rangle$  means an ensemble averaged quantity,  $U(r; \lambda)$  means  $U$  is a function of  $r$  and depends on a parameter  $\lambda$ . In this equation  $\mu^{\text{id}}$  is the ideal part of the chemical potential, acquired for the ideal gas model, and  $\mu^{\text{ex}}$  is the excess part, which are due to the interactions in the system. We can re-write the chemical potential by substituting the ideal part by its analytic form:

$$\mu_i = \mu_i^{\text{id}} + \mu_i^{\text{ex}} = k_B T \ln(\rho_i \Lambda^3) + \mu_i^{\text{ex}}. \quad (1)$$

Considering the concentration expressed in molal units, one have for a non-ideal solution:

$$\mu_i = \mu_i^{m,*} + k_B T \ln\left(\frac{m_i}{m^0} \gamma_i^m\right) = \mu_i^{m,*} + k_B T \ln\left(\frac{m_i}{m^0}\right) + \mu_i^{m,\text{ex}}, \quad (2)$$

where  $*$  means the reference state,  $m^0$  is the standard concentration of 1 mol/kg<sub>solvent</sub> and  $m_i$  is the molality of the  $i$ -th specie. Equaling equations (1) and (2),

$$\mu_i^{m,\text{ex}} = k_B T \ln(\rho_i \Lambda^3) + \mu_i^{\text{ex}} - \mu_i^{m,*} - k_B T \ln\left(\frac{m_i}{m^0}\right). \quad (3)$$

If the reference state is defined as the infinite diluted solution, i.e. an ideal solution, one has  $\gamma_{i,\infty} = 1$  and consequently  $\mu_i^{m,\text{ex}} = 0$ . Thus, from equation (2) one has

$$\mu_i^{m,*} = k_B T \ln(\Lambda^3) + \mu_{i,\infty}^{\text{ex}} + k_B T \ln\left(\frac{m^0}{m_{i,\infty}} \rho_{i,\infty}\right). \quad (4)$$

Using equation (4) in (3)

$$\begin{aligned} \mu_i^{m,\text{ex}} &= \mu_i^{\text{ex}} - \mu_{i,\infty}^{\text{ex}} + k_B T \ln\left(\frac{m^0}{m_i} \rho_i\right) - k_B T \ln\left(\frac{m^0}{m_{i,\infty}} \rho_{i,\infty}\right) \\ &= \Delta\mu_i^{\text{ex}} + k_B T \ln\left(\frac{m_{i,\infty}}{m_i} \frac{\rho_i}{\rho_{i,\infty}}\right). \end{aligned} \quad (5)$$

The number density of the  $i$ -th species can be written in terms of its molar concentration,  $M_i$ , as

$$\rho_i = N_A M_i,$$

---

<sup>a</sup>Current address: Division of Chemistry and Chemical Engineering, California Institute of Technology, Pasadena, CA 91125

where  $N_A$  is the Avogadro's number. Thus,

$$\frac{\rho_i}{m_i} = \frac{M_i N_A}{m_i}.$$

The ratio between the molar and molal concentrations for a solution containing  $n$  solutes is given by

$$\frac{M_i}{m_i} = \frac{\rho'_{\text{solution}}}{1 + \sum_{j=1}^n m_i M_{M,j}/1000},$$

in which  $M_{M,j}$  is the molar mass of  $j$ -th species (in units of  $g/mol$ ) and  $\rho'_{\text{solution}}$  is the solution mass density (in units of  $g/mL$ ). If the solute is a single salt, them one may write it as

$$\frac{M_i}{m_i} = \frac{\rho'_{\text{solution}}}{1 + mM_M/1000},$$

where  $m$  and  $M_M$  are the salt molality and molar mass, respectively. The solution density at each salt concentration can be calculated using the Pitzer equation, the details and parameters used can be found in reference Krumgalz, Pogorelsky, and Pitzer<sup>2</sup>.

Considering infinite dilution one has  $m \rightarrow 0$  and  $\rho'_{\text{solution}} \rightarrow \rho'_w$ , i.e. the mass density of pure water, one has  $\rho_{i,\infty}/m_{i,\infty} = N_A \rho'_w$ . Using these results in equation (5) one has

$$\mu_i^{m,\text{ex}} = \Delta\mu_i^{\text{ex}} + k_B T \ln \left( \frac{\rho'_{\text{solution}}}{\rho'_{w,\infty}} \right) - k_B T \ln \left( 1 + \frac{mM_M}{1000} \right). \quad (6)$$

Using

$$M_i = M_w M_{M,w} m_i,$$

where  $M_{M,w}$  and  $M_w$  are the molar mass and molar concentration of water in solution, equation (6) can be also expressed as

$$\mu_i^{m,\text{ex}} = \Delta\mu_i^{\text{ex}} + k_B T \ln \left( \frac{\rho_w}{\rho_{w,\infty}} \right), \quad (7)$$

in which  $\rho_w$  is the number density of water in the salt solution and  $\rho_{w,\infty}$  is the number density of pure water. Since  $\mu_i^{m,\text{ex}} = k_B T \ln(\gamma_i^m)$ , one has

$$k_B T \ln(\gamma_i^m) = \Delta\mu_i^{\text{ex}} + k_B T \ln \left( \frac{\rho_w}{\rho_{w,\infty}} \right).$$

For an ionic pair in solution the total excess chemical potential can be written as

$$\mu^{m,\text{ex}} = \nu_+ \mu_+^{n,\text{ex}} + \nu_- \mu_-^{n,\text{ex}},$$

in which  $\nu_i$  is the ion stoichiometric coefficient. Thus,

$$\begin{aligned} \nu_+ k_B T \ln(\gamma_+^m) + \nu_- k_B T \ln(\gamma_-^m) &= \nu_+ \Delta\mu_+^{\text{ex}} + \nu_- \Delta\mu_-^{\text{ex}} + \nu_+ k_B T \ln \left( \frac{\rho_w}{\rho_{w,\infty}} \right) + \nu_- k_B T \ln \left( \frac{\rho_w}{\rho_{w,\infty}} \right) \\ k_B T \ln([\gamma_+^m]^{\nu_+} [\gamma_-^m]^{\nu_-}) &= \sum_{i=\{+,-\}} \nu_i \Delta\mu_i^{\text{ex}} + (\nu_+ + \nu_-) k_B T \ln \left( \frac{\rho_w}{\rho_{w,\infty}} \right). \end{aligned}$$

Since the mean activity coefficient is defined as  $[\gamma_{+/-}^m]^\nu = [\gamma_+^m]^{\nu_+} [\gamma_-^m]^{\nu_-}$ , with  $\nu = \nu_+ + \nu_-$ , one has

$$\ln(\gamma_{+/-}^m) = \sum_{i=\{+,-\}} \frac{\nu_i \Delta\mu_i^{\text{ex}}}{\nu k_B T} + \ln \left( \frac{\rho_w}{\rho_{w,\infty}} \right).$$

Similarly one has for equation (6) that

$$\ln(\gamma_{+/-}^m) = \left[ \sum_{i=\{+,-\}} \frac{\nu_i \Delta\mu_i^{\text{ex}}}{\nu k_B T} \right] + \ln \left( \frac{\rho'_{\text{solution}}}{\rho'_{w,\infty}} \right) - \ln \left( 1 + \frac{mM_M}{1000} \right).$$

Therefore, using the excess chemical potential at infinite dilution and at the desired concentration it is possible to calculate the mean activity coefficient.

## II. INFINITE DILUTION

The `infinite_dilution.csv` file contains the results for hydration free energy (HFE), ion–oxygen distance (IOD), and partial molar volume (PMV) of all monovalent salts available in AmberTools. These results were obtained using the Li–Merz (LM) and Joung–Cheatham (JC) parameter sets for the SPC/E and TIP3P water models, as well as with the newly optimized parameter set.

The first column indicates the ion and all subsequent columns use a two-level header structure where:

- The first row defines the property type:
  - "HFE" (hydration free energy, in kcal/mol)
  - "IOD" (ion–oxygen distance, in Å)
  - "PMV" (partial molar volume, in Å<sup>3</sup>)
- The second row defines the model for each property:
  - "LM\_spce": Li–Merz ions with SPC/E water
  - "LM\_tip3p": Li–Merz ions with TIP3P water
  - "JC\_spce": Joung–Cheatham ions with SPC/E water
  - "JC\_tip3p": Joung–Cheatham ions with TIP3P water
  - "this\_work": the results acquired in this work
  - "exp": experimental data

The missing data points correspond to cases where the calculations did not converge or experimental data were not available.

## III. FINITE CONCENTRATION

The `mean_activity.csv` file contains experimental data for the mean activity coefficients of all salts considered in this work, along with the results obtained using the Li–Merz (LM) and Joung–Cheatham (JC) models for the SPC/E and TIP3P water models, as well as the results from the newly optimized parameter set, both with and without the non-bond fix.

The first column indicates the concentration in molal and all subsequent columns use a two-level header structure where:

- The first row defines the salt name.
- The second row defines the model for each property:
  - "LM\_spce": Li–Merz ions with SPC/E water
  - "LM\_tip3p": Li–Merz ions with TIP3P water
  - "JC\_spce": Joung–Cheatham ions with SPC/E water
  - "This work (without NBF)": the results acquired in this work using the Lorentz–Berthelot mixing rules
  - "This work (with NBF)": the results acquired after carrying out the non-bond fix procedure
  - "mac\_exp": experimental data

The missing data points correspond to cases where the calculations did not converge.

## REFERENCES

- <sup>1</sup>J. G. Kirkwood, "Statistical mechanics of fluid mixtures," **3**, 300–313.
- <sup>2</sup>B. S. Krumgalz, R. Pogorelsky, and K. S. Pitzer, "Volumetric properties of single aqueous electrolytes from zero to saturation concentration at 298.15 ÅK represented by Pitzer's ion-interaction equations," *Journal of Physical and Chemical Reference Data* **25**, 663–689 (1996).
